# Supplementary material for: Long-lived Topological Flatband Excitons in Semiconductor Moir\'e Heterostructures: a Bosonic Kane-Mele Model Platform
Source: arXiv:2403.00052 source file (2024-09-30)
Supplement: Supplementary file 1 [file SM_topological_flatband_exciton.pdf]

# Supplemental Material for
# " Long-lived Topological Flatband Excitons in Semiconductor Moiré Heterostructures: a Bosonic Kane-Mele Model Platform"

Ming Xie,[1,*] Mohammad Hafezi,[2] and Sankar Das Sarma[1,2]

[1] *Condensed Matter Theory Center, Department of Physics, University of Maryland, College Park, Maryland 20742, USA*

[2] *Joint Quantum Institute, Department of Physics, University of Maryland, College Park, Maryland 20742, USA*

## I. Details of the Bethe-Salpeter equation

The exciton problem in a moiré superlattice is treated in an approximation considering that the exciton binding energy, on the order of $\sim 100$ meV, is much larger than the moiré potential and interlayer hybridization ($\sim 10-20$ meV). We first solve the Bethe-Salpeter equation (BSE) in the absence of the moiré superlattice effects to obtain the energy dispersion and wavefunction of the lowest-energy exciton bands, i.e., the $X_1$ and $X_2$ bands, and then derive the exciton moiré Hamiltonian in the $\{|X_1\rangle, |X_2\rangle\}$ basis. The BSE for interlayer excitons takes the form,

$$(E_{\tau,c,\mathbf{k}+\alpha_c\mathbf{Q}} - E_{\tau,vl,\mathbf{k}-\alpha_v\mathbf{Q}})A^{\tau}_{S,l,\mathbf{Q}}(\mathbf{k}) + \sum_{\mathbf{k}'}\langle\tau l\mathbf{k}\mathbf{Q}|V_{sc}|\tau l\mathbf{k}'\mathbf{Q}\rangle A^{\tau}_{S,l,\mathbf{Q}}(\mathbf{k}') = \mathcal{E}^{\tau}_{S,l}(\mathbf{Q})A^{\tau}_{S,l,\mathbf{Q}}(\mathbf{k}), \tag{S1}$$

where $E_{\tau c\mathbf{k}} = \hbar^2\mathbf{k}^2/2m_c^* + E_g$ and $E_{\tau vl\mathbf{k}} = -\hbar^2\mathbf{k}^2/2m_v^* + elV_b$ are the monolayer conduction ($c$) and valence ($v$) band dispersions under the effective mass approximation; $E_g$ is the interlayer bandgap. $\tau = \pm K$ is the valley index, $l = 1, 2$ concurrently denotes the middle ($l = 1$) and the top ($l = 2$) $WSe_2$ layers. $S$ is the exciton band index. $\mathbf{Q}$ and $\mathbf{k}$ are the center-of-mass and relative momentum of the electron-hole state, $|\tau l\mathbf{k}\mathbf{Q}\rangle \equiv \hat{c}^{\dagger}_{\tau c\mathbf{k}+\alpha_c\mathbf{Q}}\hat{c}_{\tau vl\mathbf{k}-\alpha_v\mathbf{Q}}|0\rangle$. $\hat{c}^{\dagger}(\hat{c})$ is the electron creation (annihilation) operator, and $|0\rangle$ is the charge neutrality state. $\alpha_{c(v)} = m^*_{c(v)}/M$ and $M = m_c^* + m_v^*$ is the exciton effective mass. The direct Coulomb interaction matrix is given by

$$\langle\tau' l'\mathbf{k}\mathbf{Q}|V|\tau' l'\mathbf{k}'\mathbf{Q}'\rangle = -\delta_{ll'}\delta_{\tau\tau'}\delta_{\mathbf{Q},\mathbf{Q}'}\frac{2\pi e^2}{\mathcal{A}\epsilon|\boldsymbol{k}-\boldsymbol{k}'|}e^{-l|\boldsymbol{k}-\boldsymbol{k}'|d} \tag{S2}$$

where $\mathcal{A}$ is the system area, $\epsilon$ is the effective dielectric constant, and $d$ is the interlayer pacing between neighboring layers. Note that the exchange interaction which couples $+K$ and $-K$ excitons, is absent for the interlayer excitons. We have used $d = 0.67$ nm, $\epsilon = 3.8$, $m_c^* = 0.8m_e$ for $MoSe_2$ [1] and $m_v^* = 0.43m_e$ for $WSe_2$ [2]. The resulting exciton internal wavefunction for the $S = 0$ exciton branch is a real and isotropic s-wave function. The energy dispersion is parabolic $\mathcal{E}^{\tau}_l(\mathbf{Q}) \approx E_{X_l} + \hbar^2\mathbf{Q}^2/M$ at small $\boldsymbol{Q}$, where $E_{X_l} = E_g - E_{b,X_l} - elV_b$ with $E_{b,X_l}$ the binding energy of the $X_l$ exciton. Using the parameter given above, we obtain $E_{b,X_1} = 160$ meV and $E_{b,X_2} = 106$ meV, and thus $\Delta E^0 = E_{b,X_1} - E_{b,X_2} = 54$ meV.

The exciton energy dispersion, $\mathcal{E}^{\tau}_{S=0,l}(\mathbf{Q})$, and the internal wavefunction, $A^{\tau}_{S=0,l,\boldsymbol{Q}}(\boldsymbol{k})$, are used to construct the exciton moiré Hamiltonian in the next section. (From now on, we focus on $S = 0$ and drop the exciton band index $S$ for convenience.)

---

*Electronic address: mingxie@umd.edu

## II. Derivation of Exciton Moiré Hamiltonian

### A. Exciton moiré potential

We derive the exciton moiré Hamiltonian in the basis:

$$|X_l(\mathbf{Q})\rangle_\tau = \sum_{\mathbf{k}} A^\tau_{l\mathbf{Q}}(\mathbf{k})\hat{c}^\dagger_{\tau c\mathbf{k}+\alpha_c\mathbf{Q}}\hat{c}_{\tau vl\mathbf{k}-\alpha_v\mathbf{Q}}|0\rangle. \tag{S3}$$

where $\alpha_{c(v)} = m_{c(v)}/M$ with $M$ the exciton effective mass. $l = 1, 2$ for the $X_1$ and $X_2$ excitons which coincides with the layer index with $l = 1(2)$ representing the middle (top) $MX_2$ layer. $\tau$ is the valley index. $|0\rangle$ is the empty semiconductor state without any electron and hole excitations. $A^\tau_{l\mathbf{Q}}(\mathbf{k})$ is the wavefunction for electron-hole relative motion which satisfies the normalization condition $\sum_{\boldsymbol{k}} |A^\tau_{l\mathbf{Q}}(\mathbf{k})|^2 = 1$.

The exciton moiré potential for valley $+K$ is given by

$$\begin{aligned}
\mathcal{U}^+_{l,\mathbf{Q},\mathbf{Q}'} &= {}_+\langle X_l(\mathbf{Q})|\hat{U}^+|X_l(\mathbf{Q}')\rangle_+ \\
&= \sum_{\boldsymbol{k},\boldsymbol{k}'} A^{+*}_{l\boldsymbol{Q}}(\boldsymbol{k})A^+_{l\boldsymbol{Q}'}(\boldsymbol{k}')\langle 0|\hat{c}^\dagger_{+,vl\mathbf{k}-\alpha_v\mathbf{Q}}\hat{c}_{+,c\mathbf{k}+\alpha_c\mathbf{Q}}\hat{U}^+\hat{c}^\dagger_{+,c\mathbf{k}'+\alpha_c\mathbf{Q}'}\hat{c}_{+,vl'\mathbf{k}'-\alpha_v\mathbf{Q}'}|0\rangle \\
&= \sum_{\boldsymbol{k},\boldsymbol{k}'} A^{+*}_{l\boldsymbol{Q}}(\boldsymbol{k})A^+_{l\boldsymbol{Q}'}(\boldsymbol{k}')\langle 0|\hat{c}^\dagger_{+,vl\mathbf{k}-\alpha_v\mathbf{Q}}\hat{U}^+\hat{c}_{+,vl'\mathbf{k}'-\alpha_v\mathbf{Q}'}|0\rangle\delta_{\mathbf{k}+\alpha_c\mathbf{Q},\mathbf{k}'+\alpha_c\mathbf{Q}'}
\end{aligned} \tag{S4}$$

where $\hat{U}^+ = V\sum_{i,l,\boldsymbol{k}} e^{is_{i,l}\phi}\hat{c}^\dagger_{+,vl\boldsymbol{k}}\hat{c}_{+,vl\boldsymbol{k}-\boldsymbol{g}_i}$ is the Fourier transform of the $tMX_2$ valence band moiré potential in second quantized form. $\boldsymbol{g}_i$ with $i = 1, \ldots, 6$ is the moiré reciprocal lattice vector and $s_{i,l} = (-1)^{i+l-1}$ as introduced in the main text. The matrix element can be evaluated as

$$\begin{aligned}
\langle 0|\hat{c}^\dagger_{+,vl\mathbf{k}-\alpha_v\mathbf{Q}}\hat{U}^+\hat{c}_{+,vl'\mathbf{k}'-\alpha_v\mathbf{Q}'}|0\rangle &= V\sum_{i=1}^{6}\sum_{\boldsymbol{k}''} e^{is_{i,l}\phi}\langle 0|\hat{c}^\dagger_{+,vl\mathbf{k}-\alpha_v\mathbf{Q}}\hat{c}^\dagger_{+,vl\boldsymbol{k}''}\hat{c}_{\tau vl\boldsymbol{k}''-\boldsymbol{g}_i}\hat{c}_{+,vl'\mathbf{k}'-\alpha_v\mathbf{Q}'}|0\rangle \\
&= -V\sum_{i=1}^{6} e^{is_{i,l}\phi}\delta_{\mathbf{k}-\alpha_v\mathbf{Q}+\boldsymbol{g}_i,\mathbf{k}'-\alpha_v\mathbf{Q}'}
\end{aligned} \tag{S5}$$

which enforces the hole momentum conservation up to a moiré moment vector $\boldsymbol{g}_i$. Substituting Eq. S5 into S4, we obtain

$$\begin{aligned}
\mathcal{U}^+_{l,\mathbf{Q},\mathbf{Q}'} &= -V\sum_{i=1}^{6} e^{is_{i,l}\phi}\sum_{\boldsymbol{k},\boldsymbol{k}'} A^{+*}_{l\boldsymbol{Q}}(\boldsymbol{k})A^+_{l\boldsymbol{Q}'}(\boldsymbol{k}')\delta_{\mathbf{k}-\alpha_v\mathbf{Q}+\boldsymbol{g}_i,\mathbf{k}'-\alpha_v\mathbf{Q}'}\delta_{\mathbf{k}+\alpha_c\mathbf{Q},\mathbf{k}'+\alpha_c\mathbf{Q}'} \\
&= -V\sum_{i=1}^{6} e^{is_{i,l}\phi}\sum_{\boldsymbol{k}} A^{+*}_{l\boldsymbol{Q}}(\boldsymbol{k})A^+_{l\boldsymbol{Q}'}(\boldsymbol{k}+\alpha_c\boldsymbol{g}_i)\delta_{\mathbf{Q}-\boldsymbol{g}_i,\mathbf{Q}'}
\end{aligned} \tag{S6}$$

The form factor $\sum_{\boldsymbol{k}} A^{+*}_{l\boldsymbol{Q}}(\boldsymbol{k})A^+_{l\boldsymbol{Q}'}(\boldsymbol{k}+\alpha_c\boldsymbol{g}_i)$ is essentially the overlap of exciton relative wavefunctions with a relative momentum shift $\alpha_c\boldsymbol{g}_i$. We adopt the approximation that $A^+_{l\boldsymbol{Q}}(\boldsymbol{k})$ is nearly independent of $\boldsymbol{Q}$. Because $A^+_{l,0}(\boldsymbol{k})$ is real and isotropic in momentum $\boldsymbol{k}$, the overlap is identical for different directions of the shift $\alpha_c\boldsymbol{g}_i$. We denote $\tilde{V}_l \equiv V\sum_{\boldsymbol{k}} A^{+*}_{l,0}(\boldsymbol{k})A^+_{l,0}(\boldsymbol{k}+\alpha_c\boldsymbol{g}_1)$. $\tilde{V}_l$ depends on the magnitude of $\boldsymbol{g}_i$ and therefore on twist angle $\theta$, $\tilde{V}_l = \tilde{V}_l(\theta)$, as shown in Fig. 2(d) in the main text. The exciton moiré potential eventually takes the form

$$\mathcal{U}^+_{l,\mathbf{Q},\mathbf{Q}'} = -\tilde{V}_l\sum_{i=1}^{6} e^{is_{i,l}\phi}\delta_{\mathbf{Q}-\boldsymbol{g}_i,\mathbf{Q}'} \tag{S7}$$

We remark that the twist angle dependence reflects the finite size effect of excitons, which is not captured in the local approximation where exciton moiré potential is approximated by the bandgap variation.

### B. Derivation of the moiré exciton hybridization Hamiltonian

The hybridization between $X_1$ and $X_2$ excitons originates from the interlayer hybridization of their hole component residing in the $l = 1$ (middle) and $l = 2$ (top) layers. The hybridization Hamiltonian can be obtained by projecting $T$ into the exciton basis (Eq. S3), which takes the following form for valley $+K$,

$$\begin{aligned}\mathcal{T}^{+}_{\mathbf{Q},\mathbf{Q}'} &= {}_{+}\langle X_1(\mathbf{Q})|\hat{T}|X_2(\mathbf{Q}')\rangle_{+} \\ &= \sum_{\boldsymbol{k},\boldsymbol{k}'} A^{+*}_{1,\boldsymbol{Q}}(\boldsymbol{k}) A^{+}_{2,\boldsymbol{Q}'}(\boldsymbol{k}') \langle 0|\hat{c}^{\dagger}_{+,v,1,\mathbf{k}-\alpha_v\mathbf{Q}} \hat{c}_{+,c\mathbf{k}+\alpha_c\mathbf{Q}} \hat{T} \hat{c}^{\dagger}_{+,c\mathbf{k}'+\alpha_c\mathbf{Q}'} \hat{c}_{+,v,2,\mathbf{k}'-\alpha_v\mathbf{Q}'}|0\rangle \\ &= \sum_{\boldsymbol{k},\boldsymbol{k}'} A^{+*}_{1,\boldsymbol{Q}}(\boldsymbol{k}) A^{+}_{2,\boldsymbol{Q}'}(\boldsymbol{k}') \langle 0|\hat{c}^{\dagger}_{+,v,1,\mathbf{k}-\alpha_v\mathbf{Q}} \hat{T} \hat{c}_{+,v,2,\mathbf{k}'-\alpha_v\mathbf{Q}'}|0\rangle \delta_{\mathbf{k}+\alpha_c\mathbf{Q},\mathbf{k}'+\alpha_c\mathbf{Q}'} \end{aligned} \tag{S8}$$

where $\hat{T} = t\sum_{n=1}^{3} \hat{c}^{\dagger}_{+,v,1,\boldsymbol{k}} \hat{c}_{+,v,2,\boldsymbol{k}-\boldsymbol{q}_n} + h.c.$ is the Fourier transform of the $tMX_2$ interlayer hybridization term, $T(\boldsymbol{r})$, in second quantized form. The matrix element is then

$$\begin{aligned}\langle 0|\hat{c}^{\dagger}_{+,v,1,\mathbf{k}-\alpha_v\mathbf{Q}} \hat{T} \hat{c}_{+,v,2,\mathbf{k}'-\alpha_v\mathbf{Q}'}|0\rangle &= t\sum_{n}\sum_{\boldsymbol{k}''} \langle 0|\hat{c}^{\dagger}_{+,v,1,\mathbf{k}-\alpha_v\mathbf{Q}} \hat{c}^{\dagger}_{+,v,2,\boldsymbol{k}''-\boldsymbol{q}_n} \hat{c}_{+,v,1,\boldsymbol{k}''} \hat{c}_{+,v,2,\mathbf{k}'-\alpha_v\mathbf{Q}'}|0\rangle \\ &= -t\sum_{n} \delta_{\mathbf{k}-\alpha_v\mathbf{Q},\mathbf{k}'-\alpha_v\mathbf{Q}'+\boldsymbol{q}_n}\end{aligned} \tag{S9}$$

Substituting Eq. S9 in to Eq. S8, we obtain

$$\begin{aligned}\mathcal{T}^{+}_{\mathbf{Q},\mathbf{Q}'} &= -t\sum_{n}\sum_{\boldsymbol{k},\boldsymbol{k}'} A^{+*}_{1,\boldsymbol{Q}}(\boldsymbol{k}) A^{+}_{2,\boldsymbol{Q}'}(\boldsymbol{k}') \delta_{\mathbf{k}-\alpha_v\mathbf{Q},\mathbf{k}'-\alpha_v\mathbf{Q}'+\boldsymbol{q}_n} \delta_{\mathbf{k}+\alpha_c\mathbf{Q},\mathbf{k}'+\alpha_c\mathbf{Q}'} \\ &= -t\sum_{n}\sum_{\boldsymbol{k}} A^{+*}_{1,\boldsymbol{Q}}(\boldsymbol{k}) A^{+}_{2,\boldsymbol{Q}'}(\boldsymbol{k}-\alpha_c\boldsymbol{q}_n) \delta_{\mathbf{Q},\mathbf{Q}'-\boldsymbol{q}_n}\end{aligned} \tag{S10}$$

Similar to the last section, under the approximation that $A^{+}_{l,\boldsymbol{Q}}(\boldsymbol{k})$ is real and independent of $\boldsymbol{Q}$, the form factor $\sum_{\boldsymbol{k}} A^{+*}_{l,0}(\boldsymbol{k}) A^{+}_{l,0}(\boldsymbol{k}-\alpha_c\boldsymbol{q}_n)$ is real and symmetric along different $\boldsymbol{q}_n$ directions. Denoting $\tilde{T} \equiv t\sum_{\boldsymbol{k}} A^{+*}_{1,0}(\boldsymbol{k}) A^{+}_{2,0}(\boldsymbol{k} - \alpha_c\boldsymbol{q}_1)$, the exciton hybridization Hamiltonian becomes

$$\mathcal{T}^{+}_{\mathbf{Q},\mathbf{Q}'} = \tilde{T}\sum_{n} \delta_{\mathbf{Q},\mathbf{Q}'-\boldsymbol{q}_n} \tag{S11}$$

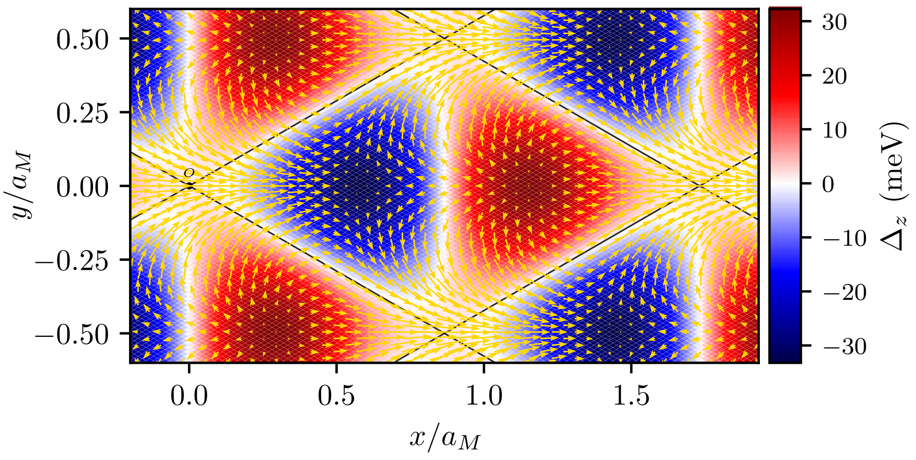


FIG. S1: Effective exciton pseudospin field $\boldsymbol{\Delta}(\boldsymbol{r})$. The arrow indicates the in-plane components, $(\Delta_x(\boldsymbol{r}), \Delta_y(\boldsymbol{r}))$, and the color indicates the z component, $\Delta_z(\boldsymbol{r})$.

where we dropped the negative sign as a matter of gauge choice. $\tilde{T}$ decreases monotonically as the twist angle increases as shown in Fig. 2(d), similar to the moiré potential term discussed in the last section.

### C. Exciton pseudo-spin skyrmion

If we define the $X_1$ and $X_2$ components as up and down pseudospins, respectively, the moiré potential and hybridization term together act as a effective exciton pseudospin magnetic field, which exhibits a skyrmion structure in real space as we show below. The effective pseudospin magnetic field (for valley +K) can be written as:

$$(\Delta_x(\boldsymbol{r}), \Delta_y(\boldsymbol{r}), \Delta_z(\boldsymbol{r})) = \left(\mathrm{Re}[\mathcal{T}^+(\boldsymbol{r})], \mathrm{Im}[\mathcal{T}^+(\boldsymbol{r})], (\mathcal{U}_1^+(\boldsymbol{r}) - \mathcal{U}_2^+(\boldsymbol{r}))/2\right) \tag{S12}$$

where $\mathcal{U}_l^+(\boldsymbol{r})$ and $\mathcal{T}^+(\boldsymbol{r})$ are the exciton moiré potential and hybridization terms. Figure S1 plots the vector field $\boldsymbol{\Delta}(\boldsymbol{r})$ with the arrow indicates the in-plane compoments and the color indicates the z-component. $\boldsymbol{\Delta}(\boldsymbol{r})$ covers the unit sphere exactly once within the moiré unit cell, with the north and south poles situated at the MX and XM positions, respectively. It therefore forms a skyrmion lattice with one skyrmion per moiré unit cell.

### D. Full moiré exciton Hamiltonian

Combining the exciton kinetic energy term, $\mathcal{E}_l(\mathbf{Q}) \approx E_{X_l} + \hbar^2\mathbf{Q}^2/M_l^*$, and the moiré potential (Eq. S7) and hybridization (Eq. S10) terms, we obtain the full exciton moire Hamiltonian (for valley $\tau = +K$)

$$\mathcal{H}^{+K}_{\mathbf{Q},\mathbf{Q}'} = \begin{pmatrix} \mathcal{E}_1(\mathbf{Q})\delta_{\mathbf{Q},\mathbf{Q}'} + \mathcal{U}^+_{1,\mathbf{Q},\mathbf{Q}'} & \mathcal{T}^+_{\mathbf{Q},\mathbf{Q}'} \\ [\mathcal{T}^+]^\dagger_{\mathbf{Q},\mathbf{Q}'} & \mathcal{E}_2(\mathbf{Q})\delta_{\mathbf{Q},\mathbf{Q}'} + \mathcal{U}^+_{2,\mathbf{Q},\mathbf{Q}'} \end{pmatrix}. \tag{S13}$$

where both $\mathcal{T}$ and $\mathcal{U}_l$ depend implicitly on twist angle. In diagonalizing the exciton moiré Hamiltonian, we adopt a hexagon centered reciprocal lattice grid, similar to Ref. 3, which respects the $C_3$ symmetry. Note that the COM momentum for the $X_1$ exciton is measured from zero momentum, while it is measured from $\boldsymbol{\kappa} = \boldsymbol{q}_1$ for the $X_2$ exciton. We have taken the parameters $(V, \phi) = (9\text{meV}, 128°)$ and $t = 18$ meV for the $\text{tWSe}_2$ [2]. The exciton moiré bandstructure is obtained by diagonalizing the Hamiltonian Eq. S13,

$$\mathcal{H}^\tau|\Phi^\tau_{n,\boldsymbol{Q}}\rangle = E^\tau_{n,\boldsymbol{Q}}|\Phi^\tau_{n,\boldsymbol{Q}}\rangle \tag{S14}$$

where $n = 0, 1, 2, \ldots$ is the band index. Figure S2 shows typical bandstructures at different twist angles, corresponding to different topological phases in addition to the $(C_0, C_1) = (-1, 1)$ phase presented in Fig.2(c) of the main text. We further plot the bandwidth $W_0$ of the lowest $n = 0$ exciton band in Fig. S3 below. The black dashed line marks the location where $W_0$ has a minimum, which we define as the location of magic angle. The red dashed line marks the location where the bandgap between the n=1 and n=2 bands closes. They deviate from each other as the vertical field $|eV_b - 2\Delta E^0|$ becomes large. The magic angle increases as the field increases. (Note that at large $|eV_b - 2\Delta E^0|$, while we still have a minimum in $W_0$, but the minimum value is no longer close to zero, so we do not consider as a magic angle.) Furthermore, the coincidence at small $|eV_b - 2\Delta E^0|$ does not occur if we artificially set the moiré

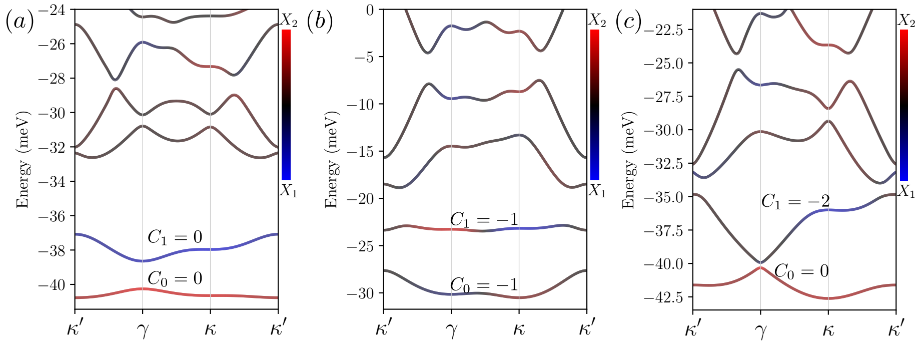


FIG. S2: Exciton moiré bandstructures at (a) $\theta = 1.5°$ and $eV_b - 2\Delta E^0 = 10$ meV, (b) $\theta = 2.5°$ and $eV_b - 2\Delta E^0 = 8$ meV, and (c) $\theta = 2.0°$ and $eV_b - 2\Delta E^0 = 18$ meV. Blue (red) line color indicates the fraction of the $X_1(X_2)$ component.

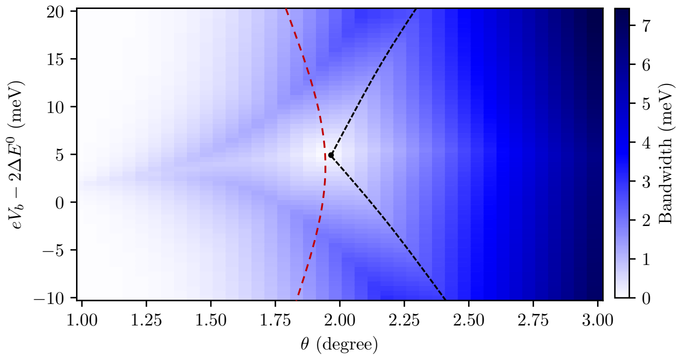


FIG. S3: Bandwidth $W_0$ of the lowest energy exciton band $n = 0$ as a function of twist angle and vertical electric field. Red dashed line marks the gap closing point between the $n = 1$ and $n = 2$ bands. Black dashed line marks the minimum in bandwidth $W_0$.

parameters to different values.

### E. Symmetry analysis

The wavefunctions at high symmetry points in the exciton mBZ are eigenstates of $C_3$ transformation,

$$C_3|\Psi^{\tau}_{n,\boldsymbol{Q}}\rangle = \eta^{C_3}_{\tau,n,\boldsymbol{Q}}|\Psi^{\tau}_{n,\boldsymbol{Q}}\rangle \tag{S15}$$

where $\eta^{C_3}_{\boldsymbol{Q},\gamma}$ is the $C_3$ eigenvalue at high-symmetry momentum. For simplicity, we define the $C_3$ transformation in the $|X_l(\boldsymbol{Q})\rangle$ basis as

$$[D_{\hat{C}_3}]_{l,\boldsymbol{Q};l'\boldsymbol{Q}'} = \delta_{ll'}\delta_{\boldsymbol{Q},\hat{C}_3\boldsymbol{Q}'} \tag{S16}$$

which factors out the spin and the orbital angular momentum of the conduction and valence band electrons inherited from their respective monolayers. In the topological phase with $(C_0, C_1) = (-1, 1)$, $\eta^{C_3}_{0,\gamma} = \eta^{C_3}_{0,\kappa} = 1$ for the lowest band ($n = 0$), and $\eta^{C_3}_{1,\gamma} = \eta^{C_3}_{1,\kappa} = e^{i2\pi/3}$ for the second lowest band ($n = 1$), $\eta^{C_3}_{n,\kappa'} = e^{-i2\pi/3}$ for both $n = 0$ and 1. We list the $C_3$ eigenvalues for different topological phases in Table I. Comparing the eigenvalues between $(-1, 1)$ and $(0, 0)$ states, we see clearly a band inversion occurring at $\boldsymbol{Q} = \boldsymbol{\gamma}$. This is true for transition between any two neighboring phases where the momentum of band inversion can be easily identified.

## III. Wannier function of the low-energy moiré exciton bands

When the low-energy moiré exciton bands are isolated from the higher energy bands, it is possible to construct localized Wannier orbitals and corresponding effective lattice models. We focus on the parameter regime where the

TABLE I: $C_3$ eigenvalues of the lowest two exciton moiré bands at different high symmetry momentum for different topological phases (labeled by the Chern number $(C_0, C_1)$). For $(0, 0)$ and $(0, -2)$ phases, we choose the positive bias sector, $eV_b - 2\Delta E^0 > 0$, as examples.

| Phases $(C_0,C_1)$ | $n = 0$ | | | $n = 1$ | | |
|---|---|---|---|---|---|---|
| | $\eta^{C_3}_{0,\gamma}$ | $\eta^{C_3}_{0,\kappa}$ | $\eta^{C_3}_{0,\kappa'}$ | $\eta^{C_3}_{1,\gamma}$ | $\eta^{C_3}_{1,\kappa}$ | $\eta^{C_3}_{1,\kappa'}$ |
| $(0, 0)$ | $\omega$ | 1 | $\omega^*$ | 1 | $\omega$ | $\omega^*$ |
| $(-1, 1)$ | 1 | 1 | $\omega^*$ | $\omega$ | $\omega$ | $\omega^*$ |
| $(-1, -1)$ | 1 | 1 | $\omega^*$ | $\omega$ | $\omega$ | 1 |
| $(0, -2)$ | $\omega$ | 1 | $\omega^*$ | 1 | $\omega$ | 1 |

lowest pair of bands are gapped from the higher bands and have Chern number $(C_0, C_1) = (-1, +1)$. We start from the trial Wannier function for the two orbitals,

$$|W_{\alpha,\boldsymbol{R}}\rangle = \frac{1}{\sqrt{N}} \sum_{n=0,1} \sum_{\boldsymbol{Q}} e^{-i\boldsymbol{Q}\cdot\boldsymbol{R}} F^n_{\alpha,\boldsymbol{Q}} |\Psi_{n,\boldsymbol{Q}}\rangle \tag{S17}$$

where $\alpha = 1, 2$ is the orbital index and $n = 0, 1$ is band index. $F_{\boldsymbol{Q}}$ is a $2 \times 2$ unitary gauge fixing matrix to be determined in the following. We focus on the $\boldsymbol{R} = 0$ site.

In the limit where the exciton hybridization is turned off, $F_{\boldsymbol{Q}}$ is diagonal and the Wannier orbitals have either $X_1$ or $X_2$ single component only. By examining the real space density of the two moiré bands,

$$\rho_n(\boldsymbol{r}) = \frac{1}{A} \sum_{\boldsymbol{Q}} |\langle \boldsymbol{r}|\Psi_{n,\boldsymbol{Q}}\rangle|^2. \tag{S18}$$

As shown in Fig. S4, $\rho(\boldsymbol{r})$ peaks at $\boldsymbol{t}_\alpha = \alpha(1/\sqrt{3}, 0)$ for the $X_{l=\alpha}$ exciton with $\alpha = 1, 2$. Assuming $n = 0(1)$ band belongs to the $X_{1(2)}$ exciton, $F_{\boldsymbol{Q}} = diag\{F^0_{1,\boldsymbol{Q}}, F^1_{2,\boldsymbol{Q}}\}$ can be obtained by requiring $F^0_{1,\boldsymbol{Q}}\langle \boldsymbol{r}|\Psi_{0,\boldsymbol{Q}}\rangle$ and $F^1_{2,\boldsymbol{Q}}\langle \boldsymbol{r}|\Psi_{1,\boldsymbol{Q}}\rangle$ to be real at $\boldsymbol{r} = \boldsymbol{t}_1$ and $\boldsymbol{r} = \boldsymbol{t}_2$, respectively, for every $\boldsymbol{Q}$.

Now we turn to the case with nonzero exciton hybridization. $F_{\boldsymbol{Q}}$ is no longer diagonal because of the mixing between $X_1$ and $X_2$ excitons. We disentangle the mixing, following the approach in Ref. 4, by considering the polarization matrix

$$\mathcal{P}_{nn'}(\boldsymbol{Q}) = \langle \Psi_{n,\boldsymbol{Q}}|\hat{P}_z|\Psi_{n',\boldsymbol{Q}}\rangle \tag{S19}$$

where $P_z \equiv |X_1\rangle\langle X_1| - |X_2\rangle\langle X_2|$. We first require that $F_{\boldsymbol{Q}}$ diagonalizes $\mathcal{P}_{nn'}(\boldsymbol{Q})$,

$$F^\dagger_{\boldsymbol{Q}} \mathcal{P}_{nn'}(\boldsymbol{Q}) F_{\boldsymbol{Q}} = \begin{pmatrix} \lambda_1 & 0 \\ 0 & \lambda_2 \end{pmatrix} \tag{S20}$$

which fixes the relative phase between the relative phase between $X_1$ and $X_2$ components. The diagonal value is ordered as $\lambda_1 > \lambda_2$ with $\lambda_\alpha$ the eigenvalue of the $\alpha$ orbital. In our calculations $\lambda_{1(2)}$ is close to $\pm 1$. We then fix the overall phase freedom by requiring $\sum_n F^\alpha_{n,\boldsymbol{Q}}\langle \boldsymbol{r}|\Psi_{n,\boldsymbol{Q}}\rangle$ to be real at $\boldsymbol{r} = \boldsymbol{t}_\alpha$ for every $\boldsymbol{Q}$. These two steps uniquely determines the unitary matrix $F_{\boldsymbol{Q}}$ from which we construct the Wannier orbitals according to Eq. S17.

The resulting Wannier orbitals are plotted in Fig.4(c-f) of the main text. They transform under $\hat{C}_3$ as

$$\hat{C}_3|W_{1,\boldsymbol{R}}\rangle = |W_{1,\boldsymbol{R}'_1}\rangle \tag{S21}$$

$$\hat{C}_3|W_{2,\boldsymbol{R}}\rangle = e^{i2\pi/3}|W_{2,\boldsymbol{R}'_2}\rangle \tag{S22}$$

where $\boldsymbol{R}'_\alpha + \boldsymbol{t}_\alpha = \hat{\mathcal{R}}_{2\pi/3}(\boldsymbol{R} + \boldsymbol{t}_\alpha)$.

While both $W_1(\boldsymbol{r})$ and $W_2(\boldsymbol{r})$ are s-wave like orbitals, they acquire a different phase under $\hat{C}_3$ transformation because of the moiré momentum shift $\boldsymbol{\kappa} = \boldsymbol{q}_1$ for the $X_2$ while no such shift for the $X_1$ exciton.

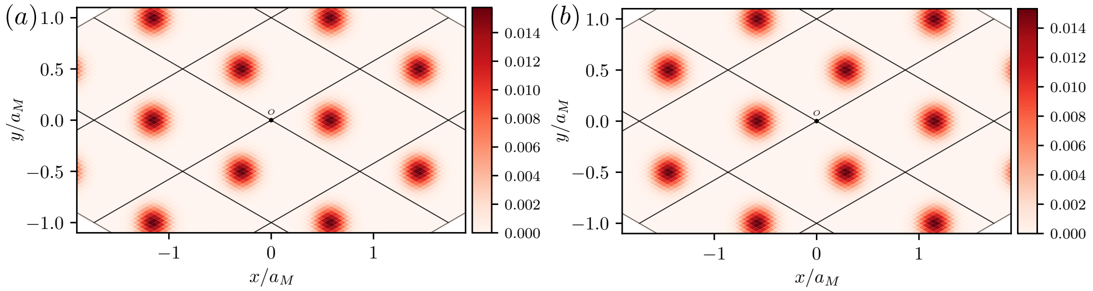


FIG. S4: Real space density of lowest exciton moiré of (a) $X_1$ and (b) $X_2$ exciton in the limit of zero hybridization ($t = 0$). The twist angle is $\theta = 1.6°$.

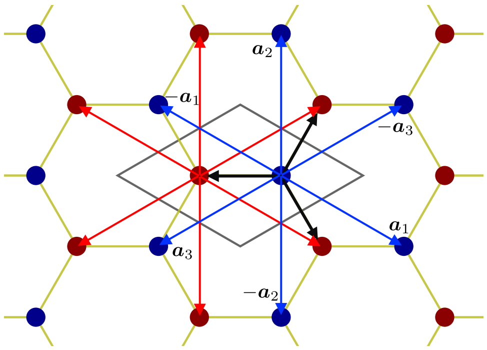


FIG. S5: Schematic illustration of the nearest neighbor (NN) and next nearest neighbor (NNN) hoppings. Black arrows represent the NN hopping between $W_1$ and $W_2$ sublattices. Blue (red) arrows represent NNN hopping between $W_1$ ($W_2$) orbitals. The black diamond outlines the $\boldsymbol{R} = 0$ moiré unit cell. $\boldsymbol{R}_1\boldsymbol{a}_1 = (-\sqrt{3}/2, 1/2)a_M$, $\boldsymbol{a}_2 = (0, 1)a_M$.

## IV. Effective Kane-Mele lattice model

In this section, we give details on the construction of the effective lattice model based on the Wannier orbitals obtained in the previous section. Again we focus on the case where the lowest pair of moiré exciton bands are gapped from higher energy bands and having Chern number $(C_0, C_1) = (-1, +1)$. The general hopping matrix element is given by

$$t_{ij}^{\alpha\alpha'} = \langle W_{\alpha,\boldsymbol{R}_i}|\mathcal{H}|W_{\alpha',\boldsymbol{R}_j}\rangle \tag{S23}$$

For small twist angle, we found that it is sufficient to keep up to 2nd nearest neighbor hopping terms, as illustrated in Fig. S5. We denote the nearest neighbor hopping, which is inter-orbital, and next nearest neighbor hopping, which is intra-orbital, as $t_m^{(1),12}$ and $t_m^{(2),\alpha\alpha}$ with $m = 1, \dots, 3$. The three NN hopping terms are

$$t_m^{(1),12} \equiv \langle W_{1,\boldsymbol{\delta}_m}|\mathcal{H}|W_{2,\boldsymbol{0}}\rangle = -\omega^{m-1}t^{(1)} \tag{S24}$$

where $\boldsymbol{\delta}_m = \{\boldsymbol{0}, -\boldsymbol{a}_3, \boldsymbol{a}_1\}$, $\omega = e^{i2\pi/3}$ and $t^{(1)}$ is the amplitude of the NN hopping. Similarly, the NNN hoppings are

$$\begin{aligned} t_i^{(2),11} &\equiv \langle W_{1,\boldsymbol{a}_m}|\mathcal{H}|W_{1,\boldsymbol{0}}\rangle = -e^{i\phi_1}t_1^{(2)} \\ t_i^{(2),22} &\equiv \langle W_{2,\boldsymbol{a}_m}|\mathcal{H}|W_{2,\boldsymbol{0}}\rangle = -e^{i\phi_2}t_2^{(2)} \end{aligned} \tag{S25}$$

where $t_\alpha^{(2)}$ and $\phi_\alpha$ are the amplitude and phase of the NNN hopping, which are parameter dependent. In the limit of zero hybridization, $T = 0$, $\phi_1 = 0$ and $\phi_2 = \kappa \cdot \boldsymbol{a}_1$ originating from the moiré momentum shift. $\phi_1$ ($\phi_2$) deviates from 0 and $\kappa \cdot \boldsymbol{a}_1$ as $T$ increases from zero. Combining the NN and NNN terms, we obtain the effective lattice model Hamiltonian (for valley +K)

$$\mathcal{H}_{eff}^{+K} = -\sum_{\alpha,i}\sum_{m=1}^{3} t^{(2)}e^{i\phi_\alpha}\hat{b}^\dagger_{\alpha,\boldsymbol{R}_i+\boldsymbol{a}_m}\hat{b}_{\alpha,\boldsymbol{R}_i} - \sum_{\alpha,i}\sum_{m=1}^{3} t^{(1)}e^{i\omega^{m-1}}\hat{b}^\dagger_{1,\boldsymbol{R}_i+\boldsymbol{\delta}_m}\hat{b}_{2,\boldsymbol{R}_i} + h.c. \tag{S26}$$

which is a generalized version of the Haldane Hamiltonian shifted in momentum space, $\mathcal{H}_{eff}^{+K}(\boldsymbol{Q}) = \mathcal{H}_{Haldane}(\boldsymbol{Q} - \boldsymbol{\kappa}')$. The Hamiltonian at valley $-K$, $\mathcal{H}_{eff}^{-K}$, can be obtained by time reversal symmetry, and together with $\mathcal{H}_{eff}^{+K}$, forms the effective Kane-Mele model. When the vertical electric field does not fully offset the difference in band alignment, we have an additional sublattice potential term in the effective lattice model,

$$\mathcal{H}_{mass,eff}^{+K} = \frac{\delta m}{2}\sum_i(\hat{b}^\dagger_{1,\boldsymbol{R}_i}\hat{b}_{1,\boldsymbol{R}_i} - \hat{b}^\dagger_{2,\boldsymbol{R}_i}\hat{b}_{2,\boldsymbol{R}_i}) \tag{S27}$$

where $\delta m$ is directly proportional to the vertical electric field as expected.

[1] S. Larentis, H. C. P. Movva, B. Fallahazad, K. Kim, A. Behroozi, T. Taniguchi, K. Watanabe, S. K. Banerjee, and E. Tutuc, Phys. Rev. B **97**, 201407(R) (2018).
[2] T. Devakul, V. Crépel, Y. Zhang, and L. Fu, Nat. Comm. **12**, 6730 (2021).
[3] B. A. Bernevig, Z.-D. Song, N. Regnault, and B. Lian, Phys. Rev. B **103**, 205411 (2021).
[4] X.-J. Luo, M. Wang, and F. Wu, Phys. Rev. B 107, 235127 (2023).
